# Supplementary material for: The dynamic nature of high pressure ice VII
Source: arXiv:2011.00875 source file (2020-11-17)
Supplement: Supplementary file 1 [file sm.pdf]

# Supplemental material:

# The dynamic nature of high pressure ice VII


Qi-Jun Ye,[1] Lin Zhuang,[1] and Xin-Zheng Li[1,2,*]

[1] *State Key Laboratory for Artificial Microstructure and Mesoscopic Physics, and School of Physics, Peking University, Beijing 100871, P. R. China*

[2] *Collaborative Innovation Center of Quantum Matter, Peking University, Beijing 100871, P. R. China*



(Dated: November 17, 2020)

In this supplemental material, we provide more technical details of our simulations and some additional discussions. Simulation details are presented in the first section, which includes the derivation of first-principles based neutral network potential, the subsequent molecular dynamic simulations, and post treatments to analyse the atomic trajectories. The second section is devoted to some additional discussions. We confirm that the proposed dynamic states are globally uniformed and hence well-defined, despite of the fact that dynamic activities are out of equilibrium. We notice that the systematic error which originates from the sampling resolution of $p_0(K)$ become significant when the dynamic field is negatively large enough. Then, we also show the map between $P$ and $s_{\text{ref}}$, the gradual transition presented with $P$, and the determination of the transition point. Numerical evidences are shown to confirm that central limit theorem is valid in the dynamically homogeneous region. Besides, we present more evidences to support the occurrence of transition, which includes the inactive component ratio, the distribution of protons displacement, the occupation of protons in components, and the decomposition of oxygens with different coordination number to protons.

## I. SIMULATION DETAILS

In handling the dynamics of bcc ice, accurate atomic potential and large simulation scale are both prerequisites. The former enables an accurate description of the chemical bond breaking process associate with proton transfers, and the latter ensures that rare events can be captured. However, high accuracy and extensive simulations are typically not compatible in practice. The proceeding technique balancing this and used in our article is the neutral network (NN) potential, which is trained based on first principles results. NN potential can offer the efficiency in a level comparable to empirical potential, enabling extensive simulations with reasonable computational costs.

### A. First principles based neutral network potential

We start with generating the inputs for the NN potential from first principles calculations. Vienna *ab initio* Simulation Package (VASP)[1,2] is used to run a series of *ab initio* molecular dynamic (MD) simulations with $T(P)$ ranging from 300 to 3,000 K (5 to 70 GPa). The

calculated configurations are selected to be representative for all involved and known phases in the $P$-$T$ region of interest, including ice VII, dynamic ice VII, superionic ice, ionic fluid, and molecular fluid. For each DFT simulation, we run 2.5-10 ps MD simulation with timestep 0.5 fs, ensuring quasi-ergodicity and sufficient sampling. To describe Van der Waals (vdW) interactions, the strongly constrained and appropriately normed (SCAN) functional was used, which outperforms other functionals with comparable computational cost in similar water systems[3]. The energy cutoff of the plane-augment wave (PAW) is set as 900 eV.

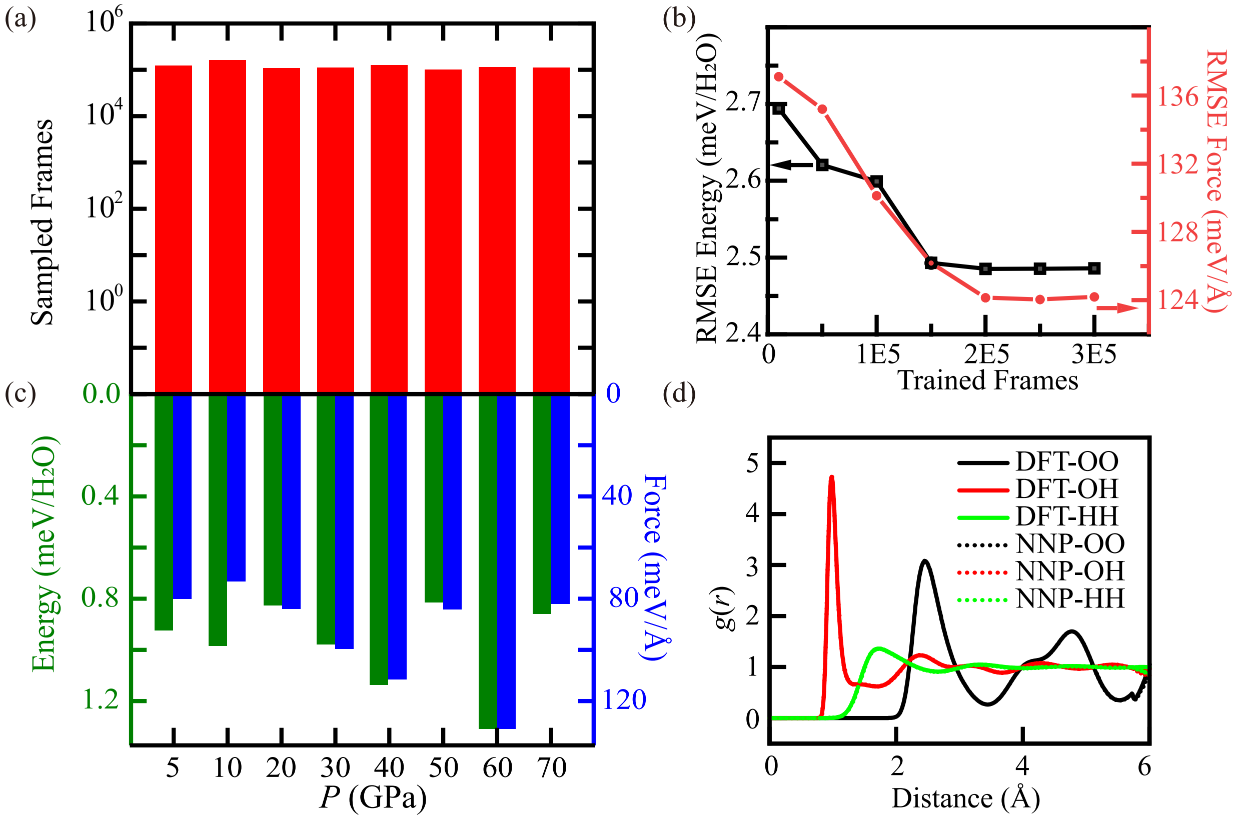


FIG. S1. (a) The condition of sampled frames in the input data sets. (b) The RMSEs of energy (black square line) and force (red circle line) with respect to trained frames. (c) The converged RMSEs of energy (green bar) and force (blue bar) at different $P$s. (d) The radial distribution function $g_{\mathrm{OO}}(r)$, $g_{\mathrm{OH}}(r)$, and $g_{\mathrm{HH}}(r)$ at 60 GPa and 2,000 K. The solid (dash) lines are the results from DFT (NN potential). The work of NN potential has been reported in Ref. [4].

By splitting the generated dataset into train and test sets, the implementation of the NN potential is done via the DeePMD-kit package[5]. The DeePMD-kit package features to preserve all the natural symmetries by building a local coordinate frame for every atom[5]. In

DeePMD, the Adam method is used to optimize the parameters of each layer of NN, as the loss function in form of

$$L(p_\epsilon, p_f, p_\xi) = p_\epsilon \Delta\epsilon^2 + \frac{p_f}{3N}\sum_i |\Delta F_i|^2 + \frac{p_\xi}{9}\left\|\Delta\xi\right\|^2 . \tag{1}$$

$N$ is the number of atoms. $\Delta\epsilon$, $\Delta F_i$, $\Delta\xi$ denote the difference between the DeePMD prediction and the training data of the energy per atom, the force on $i$-th atom, and the averaged virial tensor, respectively. Iterations were performed to reduce above loss function until the targeting criterion was met.

The input configurations are summarized in Fig. S1(a). The extensive input data sets can help eliminate the potential preconception and convince good performance at the whole region of interest. While enough configurations are trained, the NN potential approaches to a converged one. As shown in Fig. S1(b), the overall root mean square error (RMSEs) of energy and averaged force are converged above 200,000 configurations, reached the value of ~2.4 meV/$H_2O$ and ~120 meV/Å. These RMSEs are even smaller for each $P$s, shown in Fig. S1(c). The accuracy of trained potential can also be perceived from the almost merged radial distribution functions (Fig. S1(d)). It should be noted that the work on deriving this NN potential has been reported in Ref. [4].

### B. Molecular dynamics and post treatments

The MD simulations with NN potential are then preformed by using Large-scale Atomic/Molecular Massively Parallel Simulator (Lammps) with DeePMD module[5,6]. A 4×4×4 supercell containing 128 water molecule is found to be large enough to obtain converged potential energy and density, as shown in Fig. S2. For each $(T, P)$ configuration, precedent 1 ns $NPT$ and $NVT$ simulations with Nosé-Hoover thermostat are performed. As the original dynamic behaviors may be affected by the artificial bath (Nosé-Hoover thermostat), we perform sequent $NVE$ simulations to sample the atomic trajectories, wherein 1,000 snapshots sampled uniformly from each above simulation are used as the $NVE$'s initial configurations. In so doing, each $NVE$ simulations run for 10,000 steps with timestep 0.2 fs. This timescale is confirmed long enough to capture the proton transfer even at the lowest $P$=10 GPa (as the proton transfer occurs in picoseconds), and the finer timestep as 0.2 fs is selected to maximally avoid unrecorded swift transfers to farther neighbors in a

single timestep.

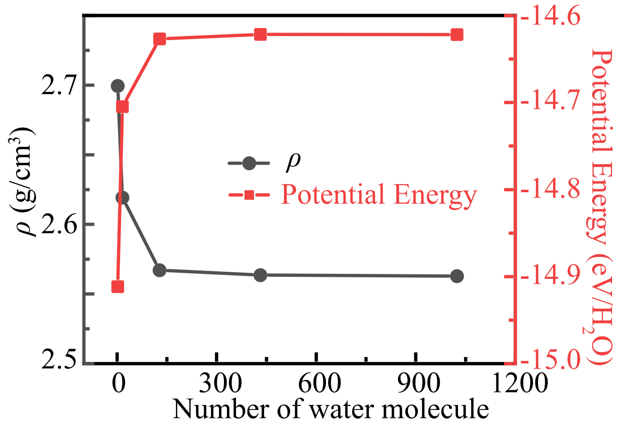


FIG. S2. Dependencies of potential energy and density on the size of the simulation cell. The result of the cell with 128 water molecule is converged.

Based on above $NVE$ simulations, we apply the concept of components to analyse the trajectories. At 500 K, when system is far from being superionic, we do not need to consider the inter component motion of oxygens (this corresponds to a much larger timescale). Considering the fact that the oxygens are localized around the bcc sites, least squares technique is performed to derive the perfect bcc structures. According to ice rule, we further derived the corresponding equivalent sites of protons (taking the equilibrium covalent position or symmetrical hydrogen bonded position of proton) and the components of protons. In our simulations, there are 256 protons and 1024 their components, which corresponds to 256 covalent sites, 256 hydrogen bonded sites, and 512 sites in another sublattice of hydrogen bonding network. Translational transfers are only related to the former 512 components, while rotational transfers are related to all components. In the article, we focus on translational transfer and do not use the latter half of components. For each timestep, we calculated the distance $d_{\text{site}}$ between the protons and the equivalent sites. A proton is determined to belong to the component which has the minimal $d_{\text{site}}$. Invalid activities exist when the protons move rapidly cross the boundary of components, similar to the case in surface hopping. In order to avoid counting this, a criterion is applied: the transfer is counted only when the proton moves far enough off the boundary (with the value 0.01 fractional coordinate of the simulation cell). An example is shown by Fig. S3. The transfer occur at about 1200 and 1550 step (shadowed region in Fig. S3) are not counted since the proton does not move

far enough off the component boundary. This criterion is consistent with the confinement condition and internal ergodicity presumed for components, which states that the atoms should explore one component for a certain time.

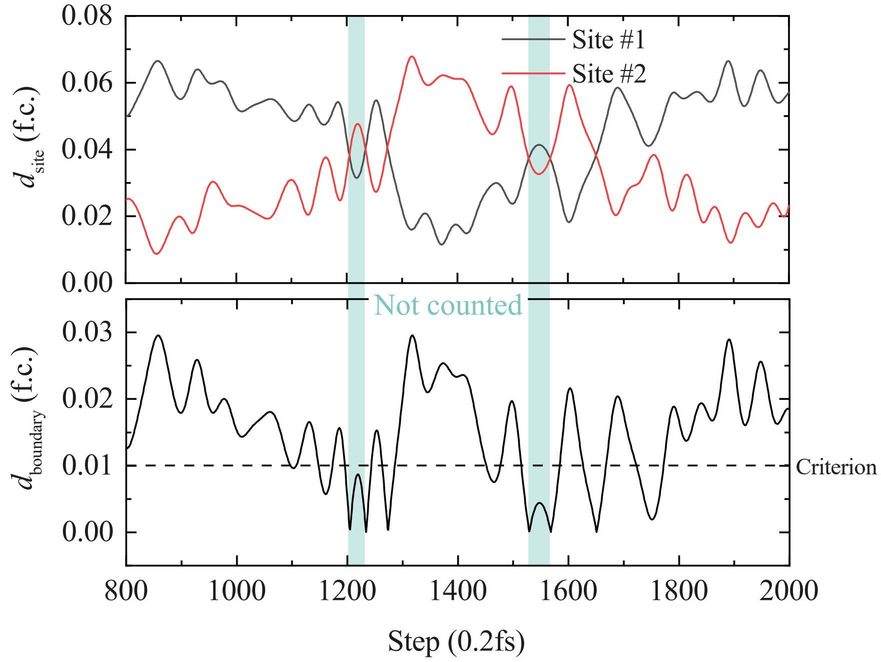


FIG. S3. A criterion with the distance off the component boundary is used to count valid activities.

In deriving $Z_{\text{ref}}$, we use the following expression

$$Z_{\text{ref}} = \sum_{(T,P)} Z_{0,(T,P)} \cdot e^{-\beta(F+PV)}. \tag{2}$$

Theoretically, the free energy $F = U + TS$ appeared here should be derived via thermodynamic integration technique. However, this requires even more extensive samplings. Regarding the computational costs, we approximate $F$ by the averaged potential energy $\langle U \rangle$ from our simulated $NPT/NVT$ snapshots.

## II. ADDITIONAL DISCUSSIONS

### A. Is the dynamic state related to rare events well-defined?

In conventionally thought thermal equilibrium, atoms oscillate around their equilibrium sites. Different from this picture, we considered rare events out of this static equilibrium.

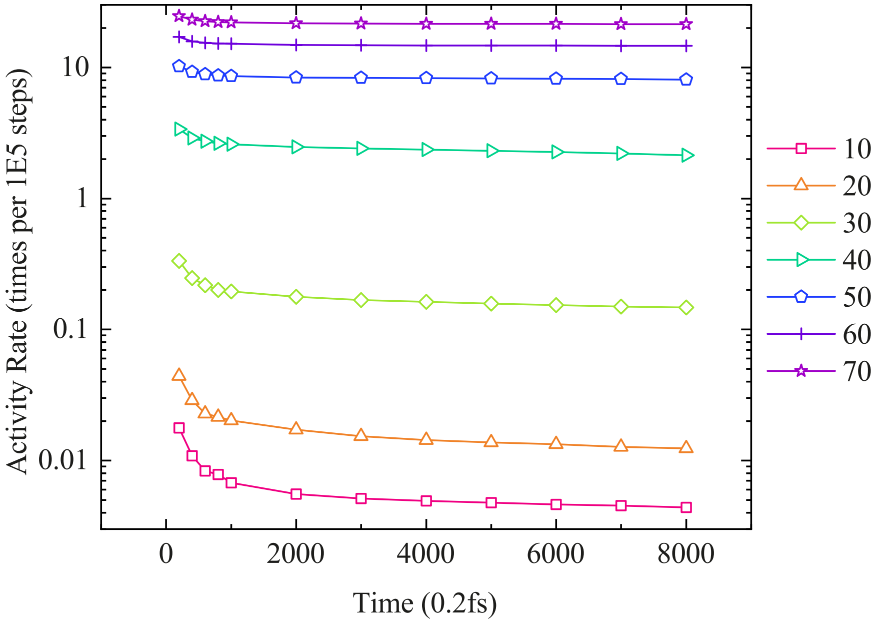


FIG. S4. The convergence of $\langle k \rangle$ on increasing $t_{\text{obs}}$.

One crucial question is that whether the system with rare events can be regarded as a uniformed state, in another word, whether these behaviors give meaningful statistics in a dynamic perspective. Here, we show the activity rate versus $t_{\text{obs}}$ curve in Fig. S4. Despite its non-equilibrium origin, the rates of proton transfers gradually saturate towards the long time limit. It means these dynamic states are well-defined with globally uniformed dynamic properties, other than ill-defined state or anomalous mixture.

### B. Systematic error emerged from the resolution of samplings

As the distribution $p_0(K)$ is sampled from MD simulations, a systematic error emerges from the resolution of samplings. If the total sampled configuration is $N$, then the undetected distribution is below a level of $\delta p_0(K) \sim 1/N$. This error be ignored when $s$ is positive or is near $s = 0$. With extensive simulations performed, $N$ can be taken so large that $\delta p_0$ is ignorable. When $s$ is negatively large, however, this error can be enhanced exponentially as $p(K) = p_0(K)\exp(-s \cdot K)$. As shown in Fig. S5(a), the distribution at 70 GPa with $s = -1$ condensates on the maximum value of $K$ observed in $p_0(K)$. This results in the reduction of $S_{\text{D}}$ (shadowed region of Fig. S5(b)), while $S_{\text{D}}$ should be monotonously increased until the bcc ice structure is changed.

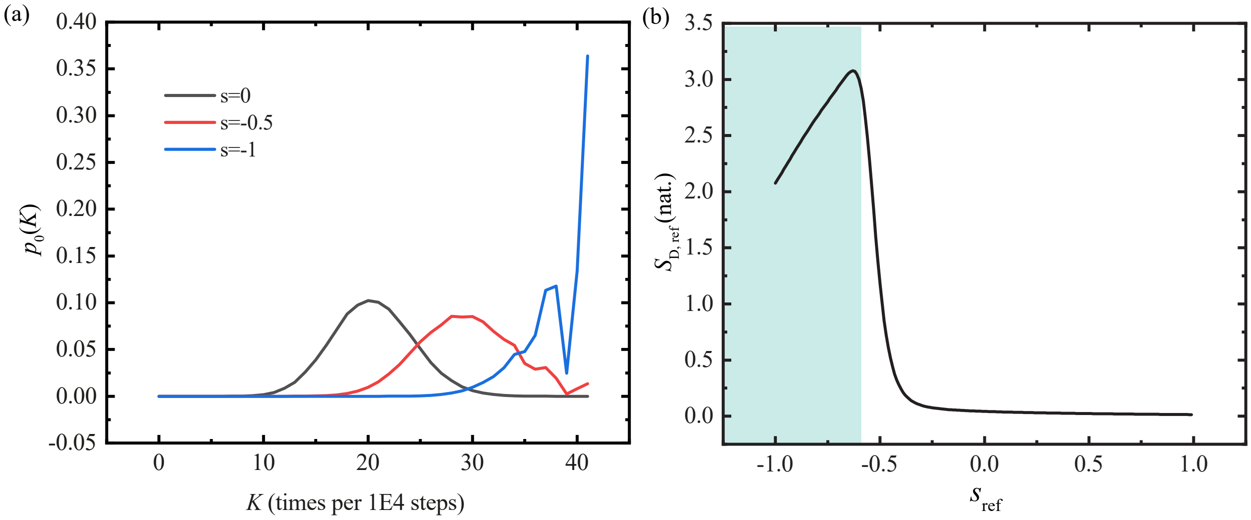


FIG. S5. (a) The $p(s, K)$ tuned by $s$ at $P = 70\ GPa$. (b) the dynamic entropy $S_{\rm D}$ versus $s_{\rm ref}$ curve. The shadowed region shows the error rooted in the resolution of probability can not be ignored.

### C. The map between $P$ and $s_{\rm ref}$

According to the equality

$$\langle A \rangle_{s=0,\ Z_{0,(T,P)}} = \langle A \rangle_{s_{\rm ref}(T,P),\ Z_{\rm ref}}, \tag{3}$$

we determine the magnitude of $s_{\rm ref}$ as a function of $(T, P)$. Fig. S6 shows their relation. $s_{\rm ref}$ is nonlinear in $P$: it varies fast at low $P$ region while it varies slowly at high $P$. It means if $P$ is used to describe the transition, the changes of $S_{\rm D}$ near the transition point will become ambiguous and rounded.

Theoretically, dynamic field $s$ is conjugated with the dynamic activity $K$ and hence is fundamental in controlling dynamic properties. The underlying truth is that $s$ measures the magnitude of dynamic constraint which is intrinsic to the mobility of system. $P$ is fundamental in controlling the volume. It can affect the proton transfer by changing the distance of neighboring oxygens. But this effect is more subtle. We show the transition revealed by $P$, in Fig. S6(b). Towards the long time limit, the curves are split into three regions, of which two are obviously corresponding to ice VII and dynamic ice VII. But the in-between region (yellow shadowed region in Fig. S6(b)) witnesses a gradual change. As no other phases are reported, it must be an intermediate or critical region. However, the wide transition range of $P$, which does not disappear with increasing simulation scale, is beyond

the knowledge of critical region in conventional thermodynamic phase transition.

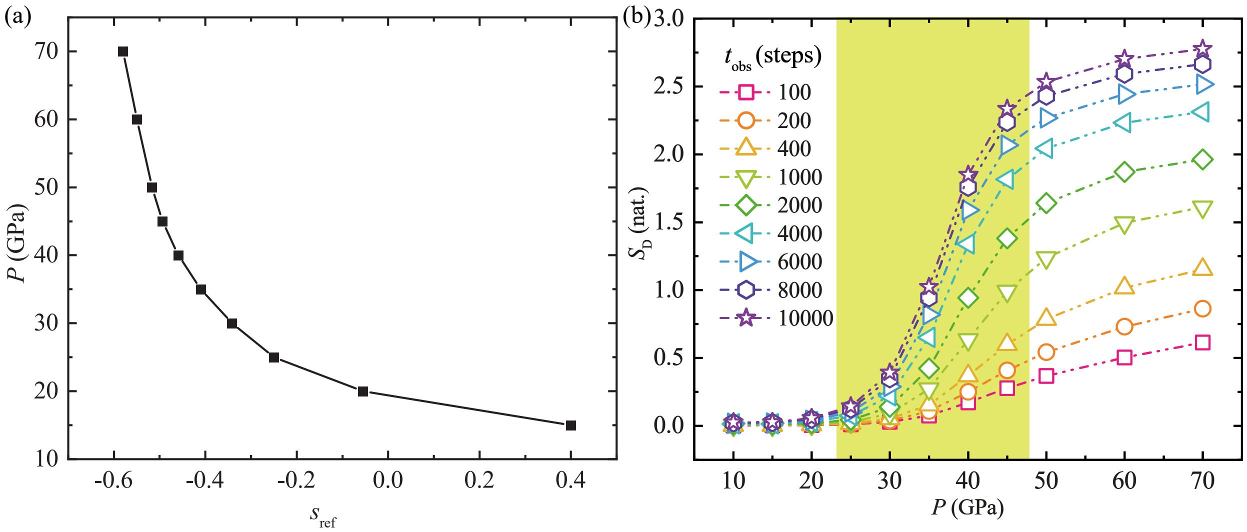


FIG. S6. (a) The map between $P$ and $s_{\mathrm{ref}}$. (b) The dynamic entropy curve with different $t_{\mathrm{obs}}$ and in perspective of $P$. The gradual transition (shadowed region) remains even at $t_{\mathrm{obs}}$ is large enough when the curves are nearly converged.

### D. Determination of the transition point

As shown in Fig. S7, the transition point $s_{\mathrm{tran}}$ at each $t_{\mathrm{obs}}$ is practically determined by the intersection of extrapolated lines of two ends. The dependencies of transition point on $t_{\mathrm{obs}}$ has been shown by exponential fitting in the main text.

### E. The validity of central limit theorem

Strictly speaking, the central limit theorem is valid only when the samples are so large and the random variables are independent with each other . The first prerequisite is fulfilled when extensive simulations are performed, while the second meets some problems. In our physical situation, the proton transfer involves two components, of which one is the starting point and another one is the destination. This makes for an instantaneous strong correlation between these two components at the moment when transfer occurs. But among all the components and the whole timescale, the activities among components are weakly correlated even can be regarded uncorrelated. Here we show the numerical evidence that $p_0(K)$ conforms to a

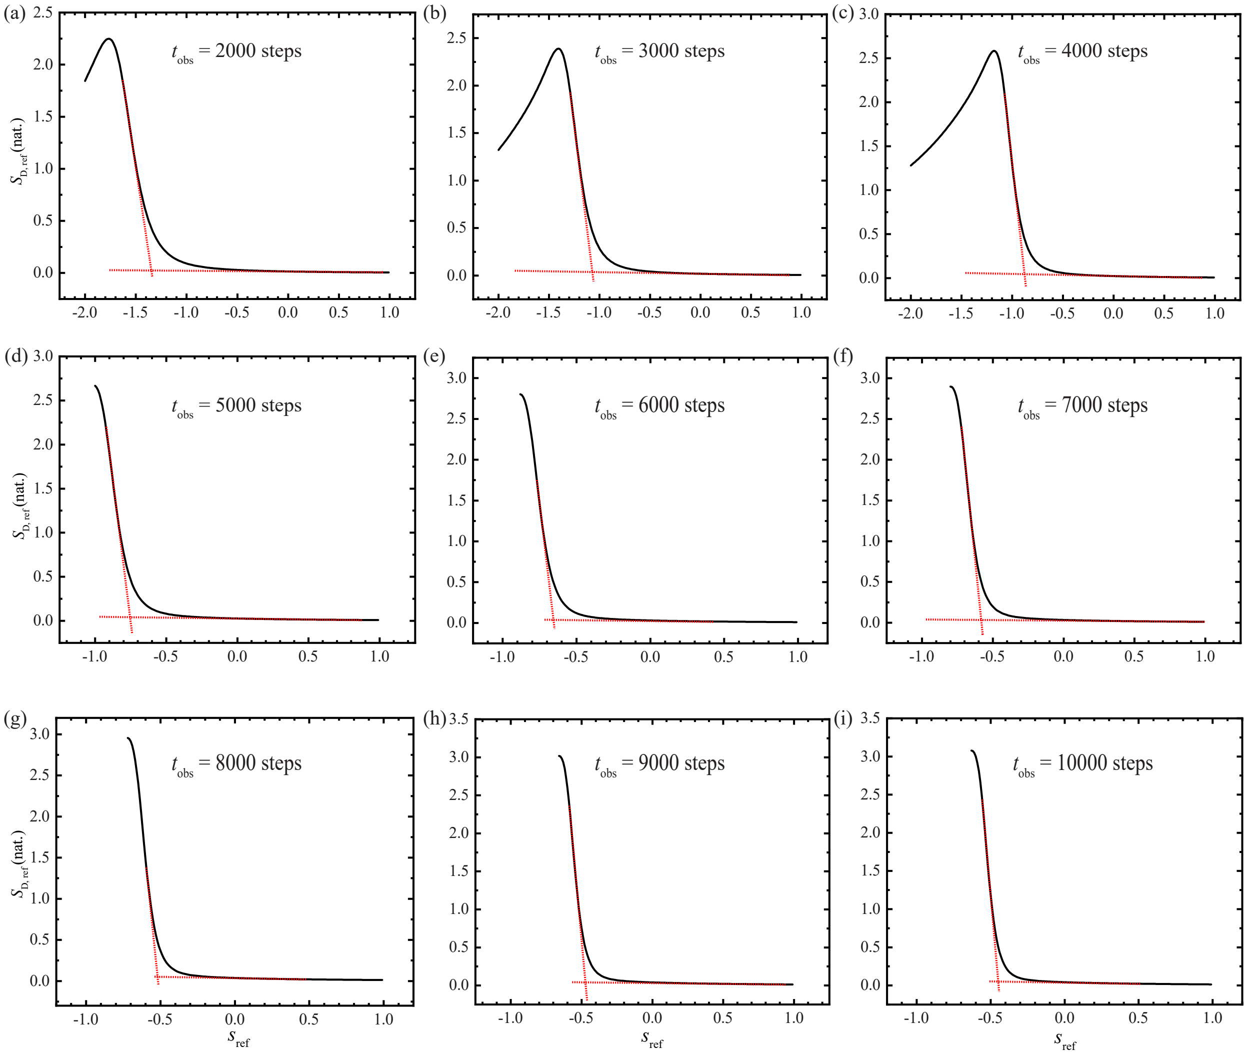


FIG. S7. The determination of transition point $s_{\mathrm{Tran}}$ at different $t_{\mathrm{obs}}$.

normalized distribution at high $P$, as the well fitted results in Fig. S8. We believe central limit theorem is still valid in this case, while more rigorous mathematical proof is awaited in future studies.

### F. Inactive component ratio

In the manuscript, we referred that the ratio of inactive component $r(t_{\mathrm{obs}})$ crucially depends on $t_{\mathrm{obs}}$. We found its $t_{\mathrm{obs}}$-dependence could be roughly fitted by a relation, as

$$r(t_{\mathrm{obs}}) = R_{\mathrm{local}} + (1 - R_{\mathrm{local}})\ e^{-t_{\mathrm{obs}}/t_0}, \tag{4}$$

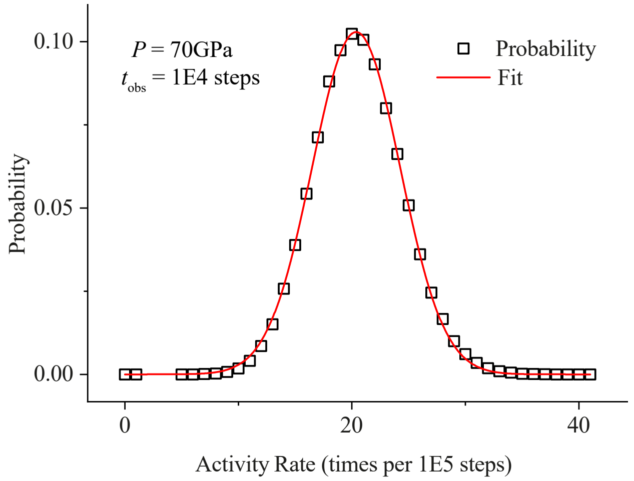


FIG. S8. The distribution $P_0(K)$ at 70 GPa and 1E4 steps (black open marks) fitted by normalized distribution (red curves).

where there are one localized part $R_{\rm local}$ receiving none temporal influence, and another diffusive part $R_{\rm diff} = 1 - R_{\rm local}$ exponentially decreased with $t_{\rm obs}$. The fitting results are shown as dashed lines in Fig. S9. Both the fitted $R_{\rm local}$ and $t_0$ present qualitative changes around our determined transition point $s_{\rm ref} = -0.37$ (Fig. S9(b)). In the active end (low $s$ and high $P$), $R_{\rm local}$ is almost one, which means few proton transfer occurs in the majority of components. It should be noted that $t_0$ might be underestimated even meaningless since low $P$ curves do not present obvious decreasing trend within our simulated timescale. While in the inactive end (high $s$ and low $P$), $R_{\rm local}$ is approaching zero and $t_0$ is lowered.

### G. Distribution of protons' displacement

We define the distribution of protons' displacement $\Delta r_i(t) = |\vec{r_i}(t) - \vec{r_i}(t + \Delta t)|$ in a certain time $\Delta t$, as

$$p_{\Delta t}(\Delta r) = \sum_i p\left(\Delta r_i\right), \ \forall t, \ \forall i = 1, \cdots, N_{\rm H}. \tag{5}$$

For a long enough $\Delta t$, $p_{\Delta t}(\Delta r)$ will be converged. There is a single peak (which can be fitted to Burr distribution) at low $P$s, while a shoulder appears at high $P$s, as shown in Fig. S10. It is the translational proton transfer which leads to the shoulder at a larger $\Delta r$. This result has been reported in Ref.[4].

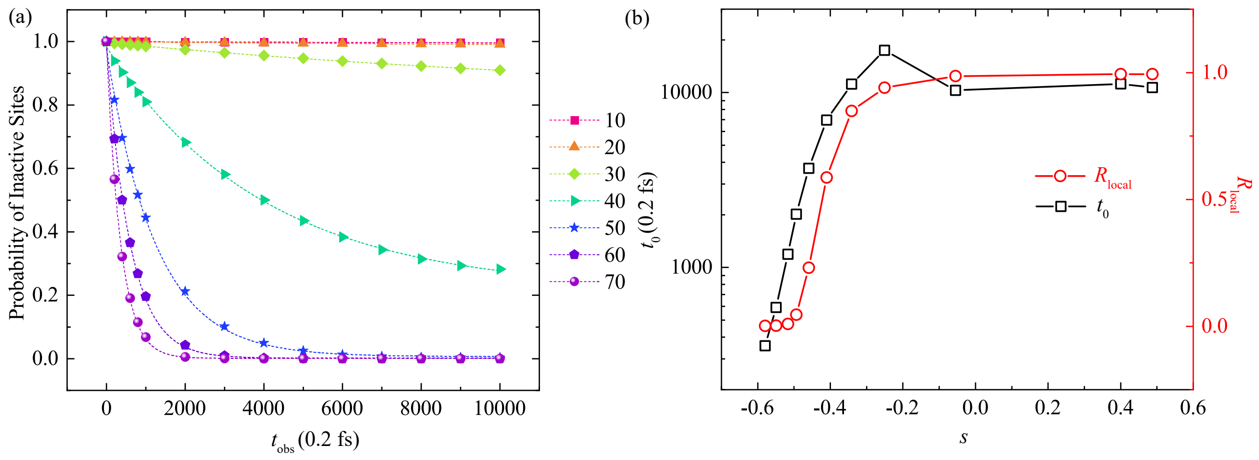


FIG. S9. (a) The inactive component ratio. Results from MD simulations are in marks and the fitting curves are in dashed lines. (b) The fitted parameter $t_0$ and $R_{\mathrm{local}}$, in black open squares and red open cricles, respectively.

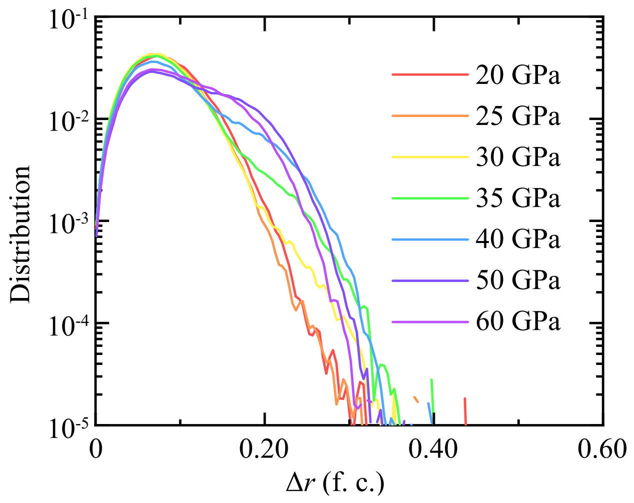


FIG. S10. The converged distribution of protons' displacement $p_{\Delta t}(\Delta r)$ at different $P$s.

### H. Occupation of protons in the components and coordination number of oxygens

Regarding the motions of protons as occupation and excitation occurred in components, we can define a descriptor of the system as

$$\{\cdots, o_i(t_{\mathrm{obs}}), \cdots\}, \tag{6}$$

where $o_i$ is the occupation state of $i$-th component at $t_{\mathrm{obs}}$. $o_i$ can only take the value as 0 or 1, since the simulated temperature is far from system being superionic or liquid (where

ice rule is broken and $o_i$ can be large than 1). We calculate its autocorrelation function, as

$$C(\Delta t) = \sum_{t_0} \sum_{i=1}^{N_{\text{comp}}} o_i(t_0) \cdot o_i(t_0 + \Delta t), \tag{7}$$

where $N_{\text{comp}}$ is the number of components. Only when transfer occurs, $o_i(t_0 + \Delta t)$ can be different from $o_i(t_0)$, bringing the reduction of correlation. As shown in Fig. S11(a), the correlation remains for a large $t_{\text{obs}}$ at low $P$s, while it rapidly decreased to 0.5 at high $P$s. The value 0.5 means the another sublattice of hydrogen bonding network is not involved. These results are consistent with the analysis in the main text.

Besides, We also present the composition of oxygens in their different coordination numbers to protons (Fig. S11 (b)). When ice rule is perfectly fulfilled, the coordination number can only be 2. The other coordination number can be observed when proton transfer occurs and ice rule is temporally violated. We find there are oxygens with 1- and 3- coordination number with moderately low probability in the region of ice VII. It means the transfer are rare and localized (the neighboring protons do not transfer simultaneously). With increased $P$s, oxygens with 1- and 3- coordination number become more frequent. And qualitatively different from low $P$ cases, oxygens with 0- and 4- coordination number (which can only be seen when the neighboring proton join the transfer) appears, implying the occurrence of collective transfer.

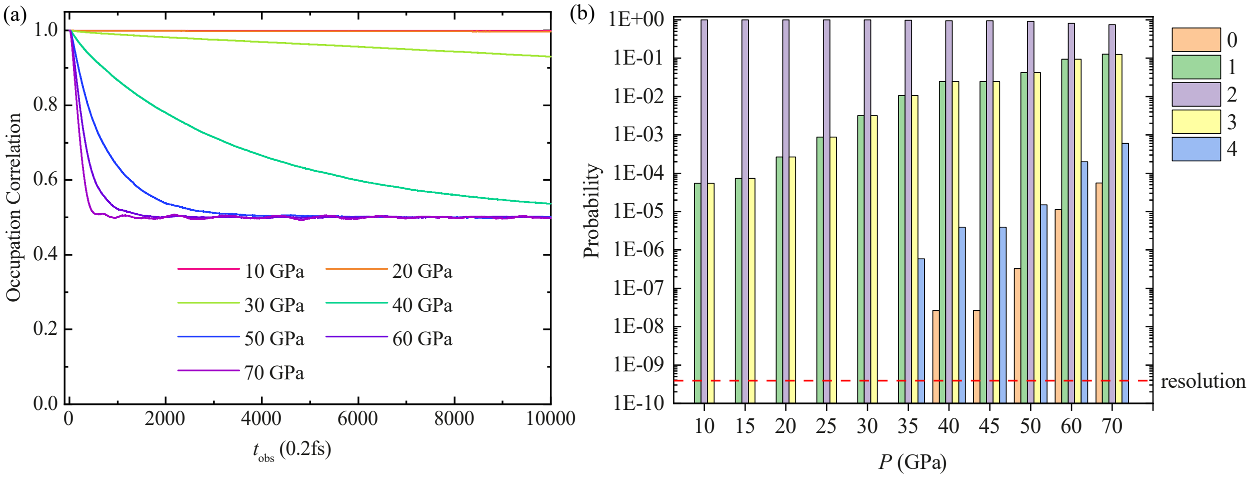


FIG. S11. (a) The autocorrelation of the occupation of protons in components. (b) The composition of oxygens in different coordination number of protons.

* xzli@pku.edu.cn

[1] G. Kresse and J. Furthmüller, Phys. Rev. B **54**, 11169 (1996).

[2] G. Kresse and D. Joubert, Phys. Rev. B **59**, 1758 (1999).

[3] J. Sun, R. C. Remsing, Y. Zhang, Z. Sun, A. Ruzsinszky, H. Peng, Z. Yang, A. Paul, U. Waghmare, X. Wu, M. L. Klein, and J. P. Perdew, Nat. Chem. **8**, 831 (2016).

[4] L. Zhuang, Q. Ye, D. Pan, and X. Li, Chinese Phys. Lett. **37**, 043101 (2020).

[5] H. Wang, L. Zhang, J. Han, and W. E, Comput. Phys. Commun. **228**, 178 (2018).

[6] S. Plimpton, J. Comput. Phys. **117**, 1 (1995).
